# Supplementary material for: Model of Cognitive Dynamics Predicts Performance on Standardized Tests
Source: arXiv:1809.02647 source file (2018-09-07)
Supplement: Supplementary file 1 [file supplementary.pdf]

# Dynamics of Performance on Standardized Tests: Supporting Information

**Nathan O. Hodas[1,2], Jacob Hunter[1], Stephen J. Young[1], and Kristina Lerman[2]**

[1]Pacific Northwest National Lab, Richland, WA 99354, USA
[2]Information Sciences Institute, University of Southern California, Marina Del Rey, CA 90292, USA

## Adversarial Depletion

Can the observed effects be attributed to random chance? To address this question, we interrogate the data in an adversarial manner to show that the observed effect is stronger than one achievable by an adversary with random data. Specifically, borrowing a page from theoretical computer science, we imagine an adversary designs a method of data summary (within certain limitations) with the goal of convincing the observer that random data is exhibiting a cognitive depletion-like effect. We will then show that this adversarial summarization of data does not create as strong of an effect in random data as what we observe, indicating that our observations are more likely to come from a real variation in performance than from random chance.

### Analysis

Given a user $u$, an event associated with that user is a 3-tuple, $(c_u, t_u, d_u)$, where $c_u$ is a binary variable indicating whether the question was correct or incorrect, $t_u$ is the time the user started work on the particular question, and $d_u$ is the length of time (in seconds) the user spent on the question. A session is a collection of events from a single user defined by an interval of time $[t_a, t_b]$. Specifically, if $s$ is a session for user $u$ defined by $[t_a, t_b]$ and $(c_u, t_u, d_u)$ is an event associated with user $u$, then $(c_u, t_u, d_u)$ is in $s$ if and only if $t_a \leq t_u \leq t_b$. We note that it is entirely possible for two intervals $[t_a, t_b]$ and $[t'_a, t'_b]$ to define the same session $S$. Thus we define a canonical interval associated with a session, specifically, given a session $S$, define

$$t_a = \min_{(c_e, t_e, d_e) \in \mathscr{S}} t_e \tag{1}$$

$$t_b = \max_{(c_e, t_e, d_e) \in \mathscr{S}} t_e + d_e. \tag{2}$$

Given a pair $x \geq y$ and a session $S$, define the sub-session $\mathscr{S}_{[x,y]}$ by

$$\{(c_e, t_e, d_e) \in S \mid t_e + x, t_e + d_e + y \leq t_b\},$$

that is, the collection of all events starting no more than $x$ seconds and ending at least $y$ seconds before the end of the session. Now for any given session $S$ (or sub-session) we define $n(S) = |S|$ and $k(S) = \sum_{(c_e, t_e, d_e) \in S} c_e$, that is the total number of events in the session and the total number of questions correct in the session, respectively. Using this notation, for $x \geq y$, we can define an adversarial scoring function on sessions $S$,

$$\mathscr{A}_{[x,y]}(S) = \begin{cases} \frac{k(S_{[x,0]})}{n(S_{[x,0]})} & \text{if } n(S_{[x,y]}) = 0 \\ \min_{(c_e, t_e, d_e) \in S_{[x,y]}} \frac{k(S_{[t_e,0]})}{n(S_{[t_e,0]})} & \text{otherwise.} \end{cases}$$

The function $\mathscr{A}_{[x,y]}$ maybe thought of as the minimum fraction of correctly answered questions starting with question inside the sub-session $S_{[x,y]}$. Reflecting this, we will refer to $[x,y]$ as the window for adversarial scoring scheme. Finally, if $\sigma \in \mathscr{S}_{n(S)}$ (that is, $\sigma$ is an element of the symmetric group on $S$) we define $\sigma S = \left\{(c_{\sigma(e)}, t_e, d_e) \mid (c_e, t_e, d_e) \in S\right\}$. In particular, if $\sigma$ is chosen uniformly at random, then $\sigma S$ is a random permutation of the correct/incorrect answers among the session $S$.

Below, we carry out a variety of statistical analyses to compare $\mathscr{A}_{[x,y]}(S)$ with $\mathscr{A}_{[x,y]}(\sigma S)$ for various choices of window and show that they are indeed different.

#### *Probability Mass Functions and $\chi^2$*

We consider, for each window $[x,y]$, two random variables $\mathscr{O}$ and $\mathscr{E}$. The random variable $\mathscr{O}$ is formed by selecting a session $S$ uniformly at random and calculating $\mathscr{A}_{[x,y]}$, while $\mathscr{E}$ is formed by selecting a session $S$ uniformly at random, then selecting $\sigma \in \mathscr{S}_{n(S)}$ uniformly and calculating $\mathscr{A}_{[x,y]}(\sigma S)$.

Table 1 compares the first three moments of $\mathscr{E}$ and $\mathscr{O}$. The first moment for $\mathscr{O}$ is always less than the first moment of $\mathscr{E}$, indicating that the observed performance is worse than one would expect in a random situation. In order to verify that these two distributions are different, we calculate the Pearson $\chi^2$ statistic between these two distributions and display the results in Table 1. For all four windows the $p$-value of the statistic is 0.0, indicating high confidence that these two distributions are indeed different.

| **window** | $[1500,900]$ | $[1800,1200]$ | $[2100,1500]$ | $[2400,1800]$ |
|---|---|---|---|---|
| $\chi^2$ | $7.75\times 10^{23}$ | $8.99\times 10^{19}$ | $1.49\times 10^{27}$ | $8.54\times 10^{54}$ |
| $p$-value | 0.0 | 0.0 | 0.0 | 0.0 |
| $\mathbb{E}[\mathscr{O}]$ | 0.483 | 0.503 | 0.515 | 0.524 |
| $\mathbb{E}[\mathscr{E}]$ | 0.518 | 0.533 | 0.542 | 0.548 |
| $\mathbb{E}\left[\mathscr{O}^2\right]$ | 0.296 | 0.310 | 0.319 | 0.325 |
| $\mathbb{E}\left[\mathscr{E}^2\right]$ | 0.315 | 0.326 | 0.333 | 0.338 |
| $\mathbb{E}\left[\mathscr{O}^3\right]$ | 0.203 | 0.211 | 0.217 | 0.220 |
| $\mathbb{E}\left[\mathscr{E}^3\right]$ | 0.207 | 0.215 | 0.220 | 0.224 |
| $\mathrm{Var}(\mathscr{O})$ | 0.0631 | 0.0571 | 0.0533 | 0.0503 |
| $\mathrm{Var}(\mathscr{E})$ | 0.0458 | 0.0416 | 0.0391 | 0.0375 |

**Table 1.** $\chi^2$ and moments of $\mathscr{E}$ and $\mathscr{O}$

### *Cumulative Distribution Function*

Next, we compare the cumulative distribution functions of $\mathscr{E}$ and $\mathscr{O}$. The cumulative distribution functions for $\mathscr{E}$ and $\mathscr{O}$ are shown in Figure 1. For all four windows, we see a similar pattern. Initially, the distribution of $\mathscr{O}$ dominates $\mathscr{E}$.[1] The gap between $\mathscr{E}$ and $\mathscr{O}$ continues to grow until approximately 0.25 and then stays steady until 0.5. Between 0.5 and 0.67 the gap between the two decreases until they cross, and then from 0.67 until 1 we see that $\mathscr{E}$ dominates $\mathscr{O}$.[2] Overall, this pattern is consistent with what we observed before: the observed performance is noticeably lower that one would expect in a truly random case.

Note that there are several prominent jumps in the cumulative probability distribution of both $\mathscr{E}$ and $\mathscr{O}$ at 0.5, 0.33, and 0.67. We suspect that these jumps correspond to testing strategies that are particularly resilient to cognitive depletion. For example, if a user were able to reliably eliminate two of the answers without much effort, and guessed randomly between the other two answers, the expected behavior would cluster around 0.5, with little variation due to depletion.

### *$z$-scores*

We compare individual sessions rather than the bulk statistics examined previously. Specifically, for a given session $S$ we compare the observed adversarial function $\mathscr{A}_{[x,y]}(S)$ with the behavior of the random adversarial function $\mathscr{A}_{[x,y]}(\sigma S)$. Given the probability mass function for $\mathscr{A}_{[x,y]}(\sigma S)$ we can calculate $\mathbb{E}\left[\mathscr{A}_{[x,y]}(\sigma S)\right]$ and $\mathrm{Var}\left(\mathscr{A}_{[x,y]}(\sigma S)\right)$ for every session $S$. From this we can calculate for every sessions $S$, the associated $z$-score

$$z_S = \frac{\mathscr{A}_{[x,y]}(S) - \mathbb{E}\left[\mathscr{A}_{[x,y]}(\sigma S)\right]}{\sqrt{\mathrm{Var}\left(\mathscr{A}_{[x,y]}(\sigma S)\right)}}.$$

This statistic should be, roughly speaking, distributed as $\mathscr{N}(0,1)$.[3] Table 2 displays the calculated mean and standard deviation of $z_S$. As in the previous analyses, the observed distribution skews lower than one would expect in the random situation, regardless of the window chosen. We also again see that this phenomenon becomes weaker as the window moves farther from the end time of the session. Additionally, we note that the variation in the $z$-score is significantly larger than expected, which would be consistent with a segment of the population exhibiting overall decreased performance.

### *Comparison Plots*

Finally, we examine the relationship between $\mathscr{A}_{[x,y]}(S)$ and $\mathbb{E}\left[\mathscr{A}_{[x,y]}(\sigma S)\right]$. We consider to what extent the expected behavior $\mathbb{E}\left[\mathscr{A}_{[x,y]}(\sigma S)\right]$ can explain the observed behavior $\mathscr{A}_{[x,y]}(S)$ via least-squares fitting. The results of the fitting are given in Table 3.

[1] This initial gap in the distribution is explained by some small proportion of the sessions where the users answered no question correctly after the window started, but had answered questions correctly at some point in time.

[2] In a similar manner as before, the final jump in cumulative probability correspond to sessions where the user answered no questions incorrectly after the window started but answered some questions incorrectly.

[3] Technically as $\mathscr{A}_{[x,y]}(\sigma S)$ has bounded support $z_S$ can not formally converge in distribution to $\mathscr{N}(0,1)$.

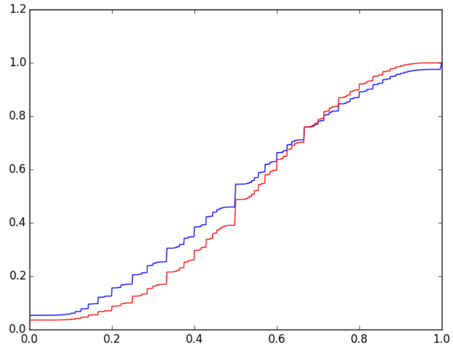


**(a)** Window $[1500, 900]$

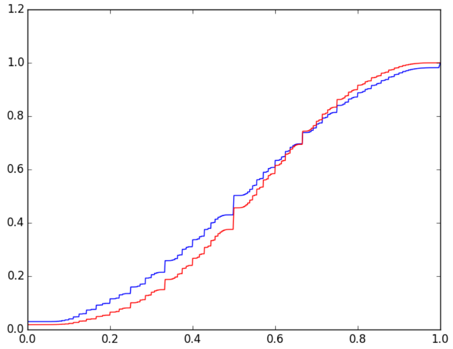


**(b)** Window $[1800, 1200]$

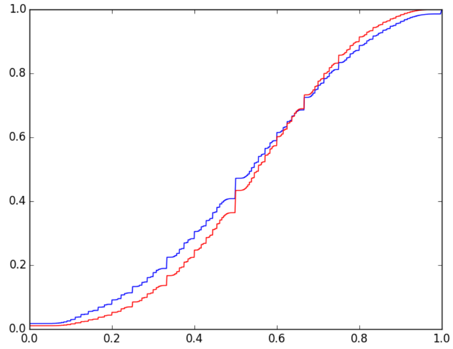


**(c)** Window $[2100, 1500]$

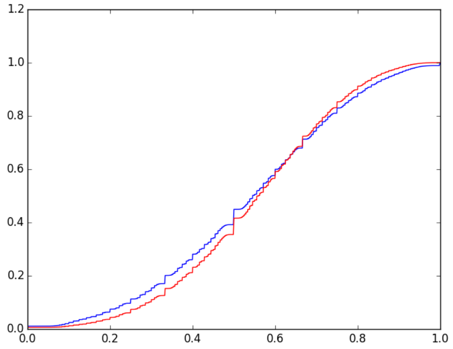


**(d)** Window $[2400, 1800]$

**Figure 1.** Cumulative Distribution Function of $\mathscr{O}$ (blue) and $\mathscr{E}$ (red).

| **window** | $[1500, 900]$ | $[1800, 1200]$ | $[2100, 1500]$ | $[2400, 1800]$ |
|---|---|---|---|---|
| $z$-score mean | $-0.164$ | $-0.121$ | $-0.0846$ | $-0.0486$ |
| $z$-score standard deviation | 1.310 | 1.316 | 1.320 | 1.318 |

**Table 2**

In Figure 2 we have plotted $\mathbb{E}\left[\mathscr{A}_{[x,y]}(\sigma)S\right]$ versus $\mathscr{A}_{[x,y]}(S)$, with the colors representing how many standard deviations $\mathscr{A}_{[x,y]}(S)$

| **window** | $[1500, 900]$ | $[1800, 1200]$ | $[2100, 1500]$ | $[2400, 1800]$ |
|---|---|---|---|---|
| $a$ | 1.111 | 1.095 | 1.078 | 1.066 |
| $b$ | $-0.0846$ | $-0.0699$ | $-0.0561$ | $-0.451$ |
| $R^2$ | 0.545 | 0.603 | 0.653 | 0.699 |

**Table 3.** $\texttt{observed} = a \times \texttt{expected} + b$

is away from $\mathbb{E}\left[\mathscr{A}_{[x,y]}(\sigma S)\right]$ (less than 1 is blue, between 1 and 2 is green, between 2 and 3 is yellow, and greater than 3 is red). Additionally, the 1-1 line is plotted (black) as well as the best-fit line (green). As the best fit line indicates, the observed values of $\mathscr{A}_{[x,y]}(S)$ skew lower than the expected values. Furthermore, significantly more observations are more than 3 standard deviations below $\mathbb{E}\left[\mathscr{A}_{[x,y]}(\sigma S)\right]$ than are 3 standard deviations above.

## Discussion

In the above analyses we see a consistent pattern: the observed distribution of performance is lower than would be expected when questions are distributed randomly in the time window. Furthermore, this pattern gets weaker as the the window moves

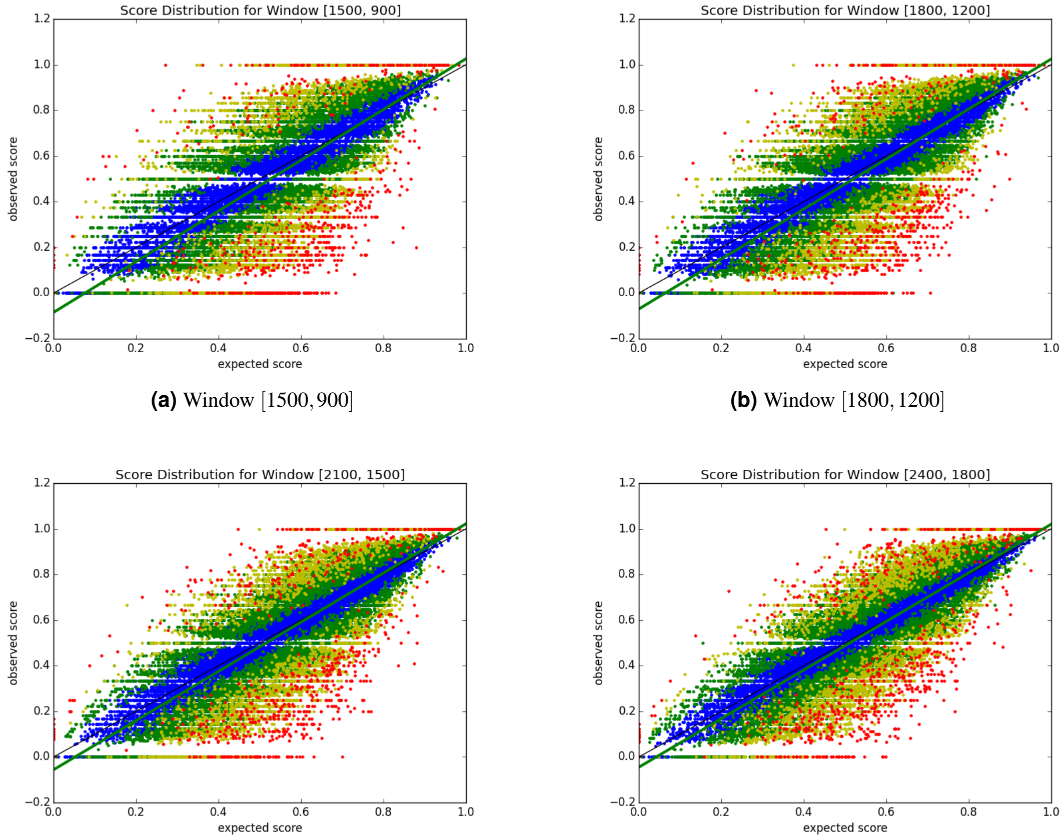


**(a)** Window $[1500, 900]$

**(b)** Window $[1800, 1200]$

**(c)** Window $[2100, 1500]$

**(d)** Window $[2400, 1800]$

**Figure 2.** Observed score in the window $[x, y]$, $\mathscr{A}_{[x,y]}(S)$, versus expected score $\mathscr{A}_{[x,y]}(\sigma S)$. Colors represent the number of standard deviations $\mathscr{A}_{[x,y]}(S)$ is away from $\mathbb{E}\left[\mathscr{A}_{[x,y]}(\sigma S)\right]$: less than 1 (blue), 1 to 2 (green), 2 to 3 (yellow), and greater than 3 (red). Additionally, the 1-1 line is plotted (black) as well as the best-fit line (green).

farther away from the end of a session. We see that the variance of the observations is greater than the randomized distribution. Thus we can conclude that there is some process that is correlated with the end of sessions which results is a decrease in overall performance.

This fits naturally into the cognitive depletion framework. Specifically, consider the following simplified model of cognitive depletion. Let $\mathscr{C}$ be the collection of all user sessions and let $\mathscr{C}' \subset \mathscr{C}$ be the subset of those sessions that will undergo cognitive depletion before terminating the session. Let $S$ be a non-cognitively depleted session, then we assume that the probability of getting an arbitrary question right is some fixed $p_S$. In contrast, for a session $S' \in \mathscr{C}'$ exhibiting cognitive depletion we say that the there are two probabilities $d_{S'} < p_{S'}$ as well as a lag parameter $\ell_{S'}$. If the user is at least $\ell_{S'}$ seconds from the end of the session, then the probability of getting a question right is $p_{S'}$, otherwise it is $d_{S'}$. Now consider an arbitrary time-slice $t$ seconds from the end of the sessions. At this time slice we have that some sessions $\mathscr{C}'_t \subset \mathscr{C}$ are in a cognitively depleted state. Furthermore if $t_1 < t_2$, then $\mathscr{C}'_{t_2} \subset \mathscr{C}'_{t_1}$. The effect of this nesting behavior will be to increase the variance and the observed value of $\mathscr{A}_{[x,y]}(\cdot)$ as the window $[x, y]$ approaches the end of the sessions. This is exactly the behavior we see in the four analyses above.

## Data Preprocessing

For any reasonable value of $n(S)$ it is computationally impractical to compute the distribution of $\mathscr{A}_{[x,y]}(\sigma S)$ naïvely as there are $n(S)!$ different permutations to consider. Instead, as the only sub-session for which the precise order of correct/incorrect matters is $S_{[x,y]}$ we may use dependent hypergeometric random variables to simulate $k(S_{[x,y]})$ and $k(S_{[y,0]})$ and then iterate over all choices of binary strings of length $n(S_{[x,y]})$ with the appropriate weight. However, as this in practice requires considering $2^{n(S_{[x,y]})}$ different binary strings, even this could be impractical depending on $n(S_{[x,y]})$. Thus, if $n(S_{[x,y]}) \geq 20$ we approximate $\mathscr{A}_{[x,y]}(\sigma S)$ by for each potential weight sampling from the space of strings with that weight. This simulation approximation

will have only a small effect on our overall results as the number of sessions requiring simulation ranges between 155 and 182, depending on the location of the window.
